# Supplementary material for: Improper Learning for Non-Stochastic Control
Source: arXiv:2001.09254 source file (2020-06-24)
Supplement: Supplementary file 9 [file F_app_checking_strong_convexity_old.tex]

%!TEX root = ../main.tex


\section{Establishing Strong Convexity\label{app:strong_convexity_check}}
	




\subsection{Proof of Proposition~\ref{prop:strong_convex_internal_controller}}

\subsubsection{Warm up: no internal controller (Proposition~\ref{prop:strong_convex_no_internal_controller})}
	We begin with consider the simpler setting where the is no stabilizing controller, that is $\Gstu^{[i]} = 0$ for all $i$. For this setting, we establish the following special case of Proposition~\ref{prop:strong_convex_internal_controller} in the main text, which we recall as follows:

	\strongconvexitynocontroller*
	Observe that the above proposition gives non-trivial strong convexity guarantees if \emph{either} the observation noise or the process noise is zero. This is crucial in deriving bounds for the LQR-setting, where $\Cst = I$ and the observation noise is zero:
	\begin{corollary} In the LQR setting, the functions $f_{t}(M)$ are $\alpha_f$-strong convex, for 
	\begin{align*}
	\alpha_f := \frac{\alphaloss \sigw^2}{(1+\|\Ast\|_{\op})^2}
	\end{align*}
	\end{corollary}

	To start, let us define the noise transfer function which maps noises $(\matw_t)$ to outputs $(\maty_t)$:
	\begin{definition}[Noise Transfer Function] Define the noise transfer function $\Gstw$ via $\Gstw^{[i]} = \Cst\Ast^{[i-1]}$ for $i > 0$, and $\Gstw^{[0]} = 0$. 
	\end{definition}
	The transfer function $\Gstw$ can be lifted to a map on sequences of noises to sequences of outputs via the Toeplitz Matrix:
	\begin{definition}[Toeplitz Matrix] Let $G = (G^{[i]}) \subset \R^{d_1\times d_2}$ be a transfer operator. We define its \emph{$(i,m,k)$-Toeplitz matrix}
	\begin{align*}
	\toep_{i,m,k}(G) := \begin{bmatrix} G^{[i]} & G^{[i+1]} & \dots & G^{[i+k-1]}\\
	0 & G^{[i]} & \dots & G^{[i+k-2]} \\
	\dots & \dots & \dots & \dots \\
	0 & 0 & \dots & G^{[i+k-m]}
	\end{bmatrix} \in \R^{d_1 m \times d_2 k}
	\end{align*}
	\end{definition}
	With these definitions in hand, we can state a bound on the strong convexity of the objective in terms of the least singular value of $\toep_{m,k}(\Gstw)$, and the variance levels $\sige^2$ and $\sigw^2$. 
	\begin{lemma}[Strong convexity, no controller, full-feedback]\label{lem:no_controller_strong_convexity} Suppose that $k \ge m$, and set 
	\begin{align*}
	\alpha_{m} = \sige^2 + \sigma_{\dimy m}(\toep_{1,m,m}(\Gstw))^2 \sigw^2.
	\end{align*} 
	Assume that Assumption~\ref{asm:strong_convexity} holds with parameter $\alphaloss$. Then, the functions $M \mapsto f_{t;k}(M) := \Exp[ \ell_t(\maty_t(M), \matu_t(M)) \mid \calF_{t-k}]$ are $\alpha_{m} \cdot \alphaloss$-strongly convex. 
	\end{lemma}
	The above lemma requires a somewhat careful computation, and is established in Section~\ref{sssec:proof_of_no_controller_strong_convexity} below.

	Observe that, in the presence of observation noise variance $\sige^2$ bounded away from zero, we can guarantee that the functions $f_{t;k}(M)$ are strongly convex without unpacking $\sigma_{\dimy m}(\toep_{1,m,k}(\Gstw))^2 \sigw^2$.  However, in our LQR setting of interest, we ought to account for the case where $\sige^2$, and thus adress the Toeplitz term. This is achieved by the following lemma, proved in Section~\ref{ssec:toeplitz_ssv}, which may be of independent interest:
	\begin{lemma}[Least Toeplitz Singular Value] \label{lem:Toeplitz_w_sigma_min}Let $m \ge k$. Then, $\sigma_{\dimy m}(\toep_{1,m,k}(\Gstw)) \ge \frac{\sigma_{\min}(\Cst)}{1+\|\Ast\|_{\op}}$. 
	\end{lemma}

	


	%Proposition~\ref{prop:strong_convex_no_internal_controller} is now a direct convexity of combining the bound from the above lemma with the guarantee from Lemma~\ref{lem:no_controller_strong_convexity}.
	

	
	

\subsubsection{Stabilized Case}

	We now generalize the above results to systems with internal stabilizing controllers.
	For a Markov operator $G$, let $G^{\top}$ denote the operator $(G^{[\top]})^{[i]} = (G^{[i]})^\top$. We first establish the following strong convexity bound in terms of relevant Toeplitz matrices:
	\begin{lemma}[Strong-Convexity for Stabilized System]\label{lem:strong-convexity_stabilized} Suppose $k \ge m+h$, and set 
	\begin{align*}
	\alpha_{m} = \left(\sige^2 + \sigma_{\dimy m}(\toep_{1,m,m}(\Gstw))^2 \,\sigw^2\right)\sigma_{\min}(\toep_{0,m,m}(\Gstutil^\top))^2,
	\end{align*} 
	where we recall $\Gstu^{[0]} = I$, and
	\begin{align*}
	\Gstutil^{[i]} = \begin{cases} 
	{}\Gstu^{[i]} & i \le h\\
	0 & i > h 
	\end{cases}
	\end{align*}
	Assume that Assumption~\ref{asm:strong_convexity} holds with parameter $\alphaloss$. Then, for $k \ge m$, the functions $M \mapsto f_{t;k}(M) := \Exp[ \ell_t(\maty_t(M), \matu_t(M)) \mid \calF_{t-k}]$ are $\alpha_{m} \cdot \alphaloss$-strongly convex. 
	\end{lemma}
	Observe that Lemma~\ref{lem:strong-convexity_stabilized} directly generalizes Lemma~\ref{lem:no_controller_strong_convexity}, where in the latter we have no internal controller, so that $\Gstutil^{[i]} = \Gstu^{[i]} = 0$ for $i > 0$. We prove this generalization in Section~\ref{sssec:proof_lemma_strong_convex_controller}. In this more general setting, we incur a term related to the Toeplitz matrix formed from the $\Gstutil$ operator. This Toeplitz operator admits the following bound, Section~\ref{ssec:toeplitz_ssv}:
		\begin{lemma}\label{lem:Toeplitz_zero_sigma_min}
		Let $G = (G^{[i]})_{i \ge 0} \in (\R^{d \times d})^{\N}$ be an arbitrary transfer operator with $G^{[0]} = I$. Then, for any $k \ge m+1$, we have
		\begin{align*}
		\sigma_{\min}(\toep_{0,m+1,k}(G)) \ge \frac{1}{2 + \sum_{i=1}^{m}\opnorm{G^{[i]}}}.
		\end{align*}
		\end{lemma}
		\begin{remark} This bound can be refined to depend on the more control-theoretic $\Hinf$-norm of $G$.
		\end{remark}
		Hence, for $k \ge m+h$ functions $f_{t;k}$ are
		\begin{align*}
		\alpha_f = \alphaloss \left(\frac{1}{2 + \sum_{i > 0}\opnorm{\Gstu^{[i]}}}\right)^2 \cdot \left(\sige^2 + \sigw^2 \left(\frac{\sigma_{\min}(\Cst)}{ 1+\|\Ast\|_{\op}^2}\right)^2\right)- \text{strongly convex},
		\end{align*}
		concluding the proof of Proposition~\ref{prop:strong_convex_internal_controller}. $\qed$
		


\subsection{Proof of Lemma~\ref{lem:no_controller_strong_convexity} (Stable Case) \label{sssec:proof_of_no_controller_strong_convexity} }

	For simplicity, let $\matu_t(M) := \matu_t(M \mid \naty_{1:t})$. 
	Since $\matu_t(M)$ is a linear function in $M$, the function $M \mapsto \lossu(\maty_t(M),\matu_t(M)) - \alphaloss \|\matu_t(M)\|_2^2$ is a convex function. Since $\alphaloss \|\matu_t(M)\|_2^2$ is a quadratic function, it then suffices to show that, for any $M$,
	\begin{align*}
	\Exp[\|\matu_t(M)\|_2^2 \mid \calF_{t-k}] \ge \alpha_{k,m} \sum_{i=0}^{m-1}\|M^{[i]}\|_{\fro}^2.
	\end{align*}
	To establish this, decompose $\maty_s$ into its conditional expectation and residuals 
	\begin{align*}
	\naty_{s\mid t-k} := \Exp[\naty_{s} \mid \calF_{t-k}], \quad 
	\naty_{s\perp t-k} := \naty_{s} - \naty_{s \mid t- k}
	\end{align*}
	Therefore, we can write
	\begin{align*}
	\iftoggle{colt}{&}{}\Exp[\|\matu_t(M)\|_2^2 \mid \calF_{t-k}] \iftoggle{colt}{\\}{}&= \Exp\left[\left\|\sum_{s = t-m-1}^t M^{[t-s]}\naty_s\right\|_2^2 \mid \calF_{t-k}\right]\\
	&= \Exp\left[\left\|\sum_{s = t-m-1}^t M^{[t-s]}(\naty_{s\mid t-k} + \naty_{s \perp t - k})\right\|_2^2 \mid \calF_{t-k}\right]\\
	&= \underbrace{\Exp\left[\left\|\sum_{s = t-m-1}^t M^{[t-s]}\naty_{s\perp t-k}\right\|_2^2  \mid \calF_{t-k}\right]}_{(i)} + \underbrace{\Exp\left[\left\|\sum_{s = t-m-1}^t M^{[t-s]}\naty_{s\mid t-k}\right\|_2^2  \mid \calF_{t-k}\right]}_{(ii)} \\
	&\quad+ \underbrace{2\Exp\left[\left\langle\sum_{s = t-m-1}^t M^{[t-s]}\naty_{s\mid t-k} , \sum_{s = t-m-1}^t M^{[t-s]}\naty_{s\perp t-k}\right\rangle  \mid \calF_{t-k}\right]}_{(iii)}
	\end{align*}
	Observe now that term $(ii)$ is greater than zero, whereas the term $(iii)$ is equal to zero, since $\naty_{s \mid t-k}$ is $\calF_{t-k}$-measurable, and $\Exp[\naty_{s\perp t-k} \mid \calF_{t-k}] = 0$. It remains to lower bound term $(i)$. We can express the expectand in $(i)$ as
	\begin{align*}
	\trace\left(\begin{bmatrix} M^{[0]\top} \\
	\dots \\
	M^{[m-1]\top}
	\end{bmatrix}^\top \underbrace{\begin{bmatrix} \Big{(}\naty_{t-i \perp t -k}\,(\naty_{t-j \perp t - k})^{\top} \Big{)}_{0 \le i,j \le m}\\ \end{bmatrix}}_{:= \matLam_{\perp t-k}} \begin{bmatrix} M^{[0]\top} \\
	\dots \\
	M^{[m-1]\top}
	\end{bmatrix}   \right).
	\end{align*}


	Therefore to prove our lower bound, it suffices show that  $\Exp[\matLam_{\perp t-k}\mid \calF_{t-k}] \succeq \alpha I$.  To establish the bound, write
	\begin{align*}
	\naty_{s \perp t-k} &= \estoch_s + \sum_{\tau = t-k-1}^{s-1}\Gstw^{[s - \tau]}\wstoch_{\tau}
	\end{align*}
	Using the the fact that the noise is mean zero and pairwise uncorrelated (Assumption~\ref{asm:noise_covariance_mart}), and using the convention $\Gst^{[i]} = 0$ for $i < 1$,
	\begin{align*}
	\Exp[\matLam_{\perp t-k}] &\succeq \sige^2\, I + \sigw^2\sum_{\tau = 1}^{k-1}  \begin{bmatrix} \Gstw^{[\tau]}\\ \Gstw^{[\tau - 1]}\\ \dots \\ \Gstw^{[\tau-(m-1)]} \end{bmatrix}\begin{bmatrix} \Gstw^{[\tau]}\\ \Gstw^{[\tau - 1]}\\ \dots \\ \Gstw^{[\tau-(m-1)]} \end{bmatrix}^{\top}\\
	&= \sige^2\, I + \sigw^2  \begin{bmatrix} \Gstw^{[1]} & \Gstw^{[2]} & \dots & \Gstw^{[k-1]}\\
	0 & \Gstw^{[1]} & \dots & \Gstw^{[k-2]} \\
	\dots & \dots & \dots & \dots \\
	0 & 0 & \dots & \Gstw^{[k-(m-1)]}
	\end{bmatrix}\begin{bmatrix} \Gstw^{[1]} & \Gstw^{[2]} & \dots & \Gstw^{[k-1]}\\
	0 & \Gstw^{[1]} & \dots & \Gstw^{[k-2]} \\
	\dots & \dots & \dots & \dots \\
	0 & 0 & \dots & \Gstw^{[k-(m-1)]}
	\end{bmatrix}^\top\\
	&:= \sige^2\, I + \sigw^2 \toep_{1,m,k}[\Gstw]\toep_{1,m,k}[\Gstw]^{\top}.
	\end{align*}
	Therefore,
	\begin{align*}
	\sigma_{\min}(\Exp[\matLam_{\perp t-k}])\ge \sige^2 + \sigw^2 \,\sigma_{\dimy m}(\toep_{1,m,k}[\Gstw])^2 \ge \sige^2 + \sigw^2 \,\sigma_{\dimy m}(\toep_{1,m,m}[\Gstw])^2 := \alpha_m,
	\end{align*}
	as needed

\subsection{Proof of \Cref{lem:strong-convexity_stabilized} (Stabilized Case) \label{sssec:proof_lemma_strong_convex_controller}}

	Again, set $\matu_t(M) = \matu_t(M \mid \Gst, \naty_{1:t},\natu_{1:t})$. When $\Gst$ includes an LDC controller, we have
	\begin{align*}
	\matu_t(M) &= \natu_{t} + \sum_{j = t-h-1}^{t}\Gstu^{[t-j]}\sum_{s=j - m - 1}^{j} M^{[j - s]}\naty_s,
	\end{align*}
	where $\Gstu^{[0]} = I$. Since affine terms are immaterial to strong convexity, it suffices show show that
	\begin{align*}
	\Exp[\|\matu_t(M) - \natu_t\|_2^2 \mid \calF_{t-k}] \ge \frac{\alpha_{f}}{\alpha_{\loss}} \|M\|_{\fro}^2,\quad \forall M.
	\end{align*}
	%
	As in the stable case, decompose
	\begin{align*}
	\naty_{s\mid t-k} := \Exp[\naty_{s} \mid \calF_{t-k}], \quad 
	\naty_{s\perp t-k} := \naty_{s} - \naty_{s \mid t- k},
	\end{align*}
	and express
	\begin{align*}
	\matu_{t\perp t-k}(M) &=  \sum_{j = t-h-1}^{t}\Gstu^{[t-j]}\sum_{s=j - m - 1}^{j} M^{[j - s]}\naty_{s \perp t-k},
	\end{align*}
	which captures the contribution of the stochastic noise terms, and define $\matu_{t \mid t-k}$ analogously. Then, analogous to the proof of Lemma~\ref{lem:no_controller_strong_convexity}, we can verify that
	\begin{align}
	\Exp[\|\matu_t(M)\|_2^2 \mid \calF_{t-k}] \ge \Exp[\|\matu_{t \perp t-k}(M)\|_2^2 \mid \calF_{t-k}]. \label{eq:wts_lb}
	\end{align}
	For $k \ge m + h$, we can express
	\begin{align*}
	\matu_{t \perp t-k}(M) &= \underbrace{\sum_{j = t-h}^{t} \Gstu^{[t-j]}\sum_{s=j - m - 1}^{j}M^{[j-s]}\estoch_{j}}_{:=\matu^{\mate}_t(M)} \\
	&\quad+ \underbrace{\sum_{j = t-h-1}^{t}\Gstu^{[t]}\sum_{s=j-m-1}^{j-1}M^{[j - s]} \sum_{\tau = t- k -1}^{s-1}\Gstw^{[s-\tau]}\wstoch_{\tau}}_{:=\matu^{\matw}_t(M)},
	\end{align*}
	where $\matu^{\mate}_t(M)$ captures the contribution of $\estoch$ and $\matu^{\matw}_t(M)$ captures the contribution of $\wstoch$. Again, from Assumption~\ref{asm:noise_covariance_mart}, we can verify that
	\begin{align*}
	\Exp[\|\matu_t(M)\|_{2}^2 \mid \calF_{t-k}] = 	\Exp[\|\matu_t^{\mate}(M)\|_{2}^2 \mid \calF_{t-k}]  + \Exp[\|\matu_t^{\matw}(M)\|_{2}^2 \mid \calF_{t-k}].
	\end{align*}
	Hence, the lower bound~\eqref{eq:wts_lb} will follow as soon as we establish the following two inequalities:
	\begin{align*}
	&\Exp[\|\matu_t^{\mate}(M)\|_{2}^2 \mid \calF_{t-k}] \ge \sige^2\cdot\sigma_{\min}(\toep_{0,m,m}(\Gstutil^\top))^2\cdot\sum_{i=0}^{m-1}\|M^{[i]}\|_{\fro}^2\\
	&\Exp[\|\matu_t^{\matw}(M)\|_{2}^2 \mid \calF_{t-k}] \ge \sigw^2\cdot\sigma_{\min}(\toep_{0,m,m}(\Gstutil^\top))^2\cdot\sigma_{m\dimy}(\toep_{1,m,m}(\Gstw))^2 \cdot \sum_{i=0}^{m-1}\|M^{[i]}\|_{\fro}^2
	\end{align*},
	where $\Gstutil$ denotes the truncated transfer operator,
	\begin{align*}
	\Gstutil^{[i]} = \begin{cases} 
	\Gstu^{[i]} & i \le h\\
	0 & i > h
	\end{cases}
	\end{align*}

	\paragraph{The contribution of $\matu_t^{\mate}(M)$:} 
	We can rewrite
	\begin{align*}
	\matu_t^{\mate}(M) &= M^{[0]}\estoch_t + (M^{[1]} + \Gstutil^{[1]}M^{[0]} )\estoch_{t-1} + (M^{[2]} + \Gstutil^{[1]}M^{[1]} + \Gstutil^{[ 2]}M^{[0]} )\estoch_{t-2}\\
	&\quad+ \dots +(M^{[m-1]}+\dots+\Gstutil^{[ m-1]}M^{[0]})\estoch_{t-(m-1)}\\
	&\qquad + \text{terms depending on } \estoch_{\tau},\, \tau < t-(m-1),
	\end{align*}
	Again, leveraging the martingale structure of the noise, the expectation of the norm $\matu_t^{\mate}(M)$ is at least that of the expectation of the contributions of $\estoch_t,\dots,\estoch_{t-(m-1)}$, which again decouple. This yields
	\begin{align*}
	\Exp[\|\matu_t^{\mate}(M)\|_2^2\mid \calF_{t-k}] &\ge \sige^2\Big\|M^{[0]}\|_{\fro}^2 + \|M^{[1]} + \Gstutil^{[1]}M^{[0]}\|_{\fro}^2 \\
	&\quad+ \dots + \|M^{[m-1]} + \dots + \Gstutil^{[ m-1]}M^{[0]}\|_{\fro}^2\Big)
	\end{align*}
	Over that the term in the paranthesis on the right hand side is equal to the trace of the following matrix:
	\begin{align}
	&(AB)^{\top}(AB), \,\text{where } \\
	&A:=
	\begin{bmatrix}
	I & 0 & 0 & \dots & 0\\
	\Gstutil^{[1]} & I & 0 & \dots & 0\\
	\Gstutil^{[2]} & \Gstutil^{[ 1]} & I & \dots & 0\\
	\dots\\
	\Gstutil^{[ m-1]} & \dots & \dots & \Gst^{[ 1]} & I
	\end{bmatrix} = \toep_{0,m,m}(\Gstutil^{\top})^{\top},\quad B := \begin{bmatrix} M^{[0]}\\
	M^{[1]}\\
	\dots\\
	M^{[m-1]}
	\end{bmatrix} \label{eq:ab_matrices}
	\end{align}
	where for a transfer operator $G$, $G^\top$ is the operator $(G^\top)^{[i]}= (G^{[i]})^\top$. 
	Hence,
	\begin{align*}
	\Exp[\|\matu_t^{\mate}(M)\|_{2}^2\mid \calF_{t-k}] &\ge \trace((AB)^{\top}(AB)) \\
	&\ge \sige^2\cdot\|B\|_{\fro}^2 \,\sigma_{\min}(A)^2\\
	&= \sige^2\cdot\sigma_{\min}(A)^2\cdot\sum_{i=0}^{m-1}\|M^{[i]}\|_{\fro}^2\cdot\\
	&= \sige^2\cdot\sigma_{\min}(\toep_{0,m,m}(\Gstutil^\top))^2\cdot\sum_{i=0}^{m-1}\|M^{[i]}\|_{\fro}^2
	\end{align*}
	\paragraph{The contribution of $\matu_t^{\matw}(M)$:}
	 We have that
	\begin{align*}
	\matu_t^{\matw} &:= \left(M^{[0]} \Gstw^{[1]}\right)\wstoch_{t-1} +\left(M^{[0]}\Gstw^{[2]} + \Gstutil^{[1]}M^{[0]}\Gstw^{[1]} +  M^{[1]}\Gstw^{[1]} \right)\wstoch_{t-2}\\
	&+ \Big(M^{[0]}\Gstw^{[3]} + \Gstutil^{[2]}M^{[0]}\Gstw^{[1]} + \Gstutil^{[1]}M^{[0]}\Gstw^{[2]}  \\
	&\qquad+  \Gstutil^{[1]} M^{[1]}\Gstw^{[1]} + M^{[1]}\Gstw^{[2]} + M^{[2]}\Gstw^{[1]} \Big)\wstoch_{t-3}\\
	&\quad+ \dots + (M^{[0]}\Gstw^{[m]} + \dots + M^{[m-1]}\Gstw^{[1]})\wstoch_{t-m} \\
	&\quad+ \text{ terms depending on } \wstoch_{\tau}, \, \tau < t-m.
	\end{align*} 
	Hence, 
	\begin{align*}
	&\Exp[\|\matu_t^{\matw}\|_2^2 \mid \calF_{t-k}] \\&\ge \sigw^2\left\|\underbrace{M^{[0]} \Gstw^{[1]}}_{= Z^{[1]}}\right\|_{\fro}^2 +\sigw^2\left\|\underbrace{M^{[0]}\Gstw^{[2]} + \Gstutil^{[1]}M^{[0]}\Gstw^{[1]} +  M^{[1]}\Gstw^{[1]}}_{= Z^{[2]}} \right\|_{\fro}^2 \\
	&+ \sigw^2\left\|\underbrace{M^{[0]}\Gstw^{[3]} + \Gstutil^{[2]}M^{[0]}\Gstw^{[1]} + \Gstutil^{[1]}M^{[0]}\Gstw^{[2]}  +  \Gstutil^{[1]} M^{[1]}\Gstw^{[1]} + M^{[1]}\Gstw^{[2]} + M^{[2]}\Gstw^{[1]}}_{=Z^{[3]}} \right\|_{\fro}^2 \\
	&\quad+ \dots +\sigw^2 \left\|\underbrace{M^{[0]}\Gstw^{[m]} + \dots + M^{[m-1]}\Gstw^{[1]}}_{Z^{[m]}}\right\|_{\fro}^2.
	\end{align*}
	With the $Z^{[i]}$ notation, we have
	\begin{align*}
	\Exp[\|\matu_t^{\matw}\|_2^2 \mid \calF_{t-k}] \ge  \sigw^2 \sum_{i=1}^{m} \|Z^{[i]}\|_{\fro}^2
	\end{align*}
	Let us now carefully unpack this above sum. Let $A$ and $B$ be the matrices from Eq.~\eqref{eq:ab_matrices}, and let $C^{[i]}$ denote the $i$-th block in their product; e.g. $C^{[1]} = M^{[0]}$, $C^{[2]} = M^{[1]} + \Gstutil^{[1]}M^{[0]}$, and so on. Then,
	\begin{align*}
	Z^{[i]} = \sum_{j=1}^{i} C^{[j-i+1]}\Gstw^{[j]}.
	\end{align*}
	In matrix form
	\begin{align*}
	\begin{bmatrix}
	Z^{[1]} & 
	Z^{[2]}
	& \dots &
	Z^{[m]} \end{bmatrix} = \begin{bmatrix} C^{[1]} & C^{[2]} & \dots & C^{[m]}\end{bmatrix}\toep_{1,m,m}(\Gstw),
	\end{align*}
	whcih gives
	\begin{align*}
	\sum_{i=1}^m\|Z^{[i]}\|_{\fro}^2 \ge \sigma_{m\dimy}(\toep_{1,m,m}(\Gstw))^2 \sum_{i=1}^m \|C^{[i]}\|_{\fro}^2.
	\end{align*}
	Moreover, in the bound on $\matu_t^{\mate}$, we in fact established that
	\begin{align*}
	\sum_{i=1}^m \|C^{[i]}\|_{\fro}^2 \ge  \sigma_{\min}(\toep_{0,m,m}(\Gstutil^\top))^2\cdot\sum_{i=0}^{m-1}\|M^{[i]}\|_{\fro}^2.
	\end{align*}
	Putting things together, we have
	\begin{align*}
	\Exp[\|\matu_t^{\matw}\|_2^2 \mid \calF_{t-k}] \ge \sigw^2\, \sigma_{m\dimy}(\toep_{1,m,m}(\Gstw))^2\,\sigma_{\min}(\toep_{0,m,m}(\Gstutil^{\top}))^2\sum_{i=0}^{m-1}\|M^{[i]}\|_{\fro}^2
	\end{align*}


	
\subsection{Least Singular Values of Toeplitz Matrices\label{ssec:toeplitz_ssv}}

	To establish lower bounds on the least singular values of relevant Toeplitz matrices, our proof strategy is to reduce to lower bounding the smallest singular value of a certain  ``power-Toeplitz matrix'':
	\begin{definition}[Power-Toeptliz Matrices]\label{defn:power_toep}
	For square matrices $A$, define its associated \emph{power-Toeplitz} matix
	\begin{align}
	\powtoep_m(A) := \begin{bmatrix} I & A & A^2 & \dots & A^{m-1}\\
	0 & I & A & \dots & A^{m-2} \\
	\dots \\
	0 & 0 & 0 & \dots & I
	\end{bmatrix} \label{eq:pow_toep_def}
	\end{align}
	\end{definition}
	The advantage of this strategy is that $\sigma_{\min}(\powtoep_m(A))$ admits the following simple lower bound:
	\begin{claim}[Smallest eigenvalue of Power Toeplitz Matrices]\label{claim:pow_toep_sigma_min} For any square $A \in \R^{d \times d}$, 
	\begin{align*}
	\sigma_{\min}(\powtoep(A)) \ge (1 + \|A\|_{\op})^{-1}.
	\end{align*}
	\end{claim}
	\begin{proof}
	It suffices to show that $\|\powtoep(A)^{-1}\|_{\op} \le 1 + \|A\|_{\op}$. 
	We can verify by direct computation that 
	\begin{align*}
	\powtoep(A)^{-1} = \begin{bmatrix} I & -A & 0 & 0 & \dots & 0\\
	0 & I & - A &  0 & \dots & 0\\
	\dots \\
	0 & 0 & \dots &0& 0 & I\end{bmatrix}.
	\end{align*}
	Hence $\powtoep(A)^{-1}$ is the sum of two matrices: the identity in $\R^{md}$, and an upper triangular block-band  matrix with $-A$ on the block-diagonal band. The first matrix has norm $1$ and the second has norm $\|A\|_{\op}$. By the triangle inequality, $\|\powtoep(A)^{-1}\|_{\op} \le 1 +\|A\|_{\op}$. 
	\end{proof}
\subsubsection{Proof of Lemma~\ref{lem:Toeplitz_w_sigma_min}}

	Let us lower bound $\sigma_{\dimy m}(\toep_{1,m,k}(\Gstw))$ in terms of $\sigma_{\min}(\powtoep_m(\Ast))$. Observe that if $A$ is an $p \times p$ submatrix of a matrix $B$, then $\sigma_{p}(B) \ge \sigma_{\min}(A)$. Thus
	\begin{align*}
	\sigma_{\dimy m}(\toep_{1,m,k}(\Gstw)) &\ge \sigma_{\min}(\toep_{1,m,m}(\Gstw))\\
	&= \sigma_{\min}\left(\begin{bmatrix} \Cst & \Cst \Ast & \dots & \Cst\Ast^{m-2}\\
	0 & \Cst & \dots & \Cst\Ast^{m-3} \\
	\dots & \dots & \dots & \dots \\
	0 & 0 & \dots & \Cst
	\end{bmatrix}\right)\\
	&= \sigma_{\min}\left(\Diag(\underbrace{\Cst,\dots,\Cst}_{\text{m times}} ) \cdot \powtoep_m(\Ast) \right)\\
	&\ge \sigma_{\min}(\Cst)\cdot\sigma_{\min}\left(\powtoep_m(\Ast)\right).
	\end{align*}
	By Claim~\ref{claim:pow_toep_sigma_min}, the last line is at least $\sigma_{\min}/(1+\|\Ast\|_{\op})$, as needed.
	\qed
\subsubsection{Proof of Lemma~\ref{lem:Toeplitz_zero_sigma_min}}

	Again, it suffices to prove that $\sigma_{\min}(\toep_{0,m+1,m+1}(G)) \ge \frac{1}{2 + \sum_{i=1}^{m}\opnorm{G^{[i]}}}$.
	%
	To prove this, we into the \emph{nilpotent dilation}, which allows us to represent the first $m$ matrices of an arbitrary transfer operator as the transfer function of a finite-order LDS (which from which we can then extract a power-Toeplitz matrix) :
	
	\begin{definition}Define the \emph{nilpotent dilation} of $G$ via 
	\begin{align*}
	\nilp_{m}(G) := \begin{bmatrix} 0 & I & G^{[m]} & G^{[m-1]} & \dots & \dots &G^{[1]} \\
	0 & 0 & I & 0 & 0 & \dots & 0 \\
	0 & 0 & 0 & I & 0 & \dots & 0 \\
	\dots
	\end{bmatrix} \in \R^{d(m+2)\times d (m+2)}
	\end{align*}
	\end{definition}
	To use the nilpotent dilation to represent $G$ as corresponding to an LDS, we first obtain an expression for its powers:
	\begin{claim}[Powers of nilpotent dilation]\label{claim:nilp_power}
	Let $1 \le i \le m$. Then
	\begin{align*}
	\nilp_{m}(G)^{i} = \begin{bmatrix} 0 & 0 & \dots I & G^{[m]} & G^{[m-1]} & \dots & \dots &G^{[i]} \\
	0 & 0 & \dots & I & 0 & 0 & \dots & 0 \\
	0 & 0 & \dots &0 & I & 0 & \dots & 0 \\
	\dots
	\end{bmatrix}
	\end{align*}
	\end{claim}
	As a consequence we can verify the following block-matrix identity:
	\begin{claim}[Representing transfer operator as LDS]\label{claim:LDS_nilpotent}
	 For $j \in [m+2]$, let $E_{j;d} \in \R^{(m+2)d \times d}$ denote the matrix with $m+2$ blocks of $d \times d$ with $I_d$ in the $j$-th block. Set $L = E_{1;d}^\top$ and $R = E_{1;d} + E_{m+2;d}$. Then, for $i \in \{0,\dots,m\}$,
	 \begin{align*}
	 L \,\cdot\,\nilp_m(G)^i \,\cdot\,R = \begin{cases} G^{[i]} & i \in [m]\\
	 I & i = 0
	 \end{cases},
	 \end{align*}
	 where $\nilp(G)^0$ is understood as the identity on $\R^{(m+2)\times d}$.
	\end{claim}
	In other words, if $\widetilde{G}$ is the transfer operator  associated with the system $(A,B,C,D) = (\nilp_m(G), R,L,0)$, then $\widetilde{G}^{[i]} = G^{[i-1]}$ for $i \in [m+1]$. 
	\begin{proof}
	First, consder $i \in [m]$. From Claim~\ref{claim:nilp_power}, we can verify
	\begin{align*}
	E_{1;d}^\top(\nilp_m(G)^i) E_{m+2;d} = G^{[p]} \quad \text{and} \quad
	E_{1;d}^\top(\nilp_m(G)^i) E_{1;d} = 0.
	\end{align*}
	These imply that $E_{1;d}^\top (\nilp_m(G)^p) (E_{1;d} + E_{m+2;d}) = G^{[i]}$. On the other hand, for $\nilp_m(G)^0 = I_{d(m+2)}$, we have $E_{1;d}^\top (I_{d(m+2)}) (E_{1;d}^\top + E_{m+2;d}) = E_{1;d}^\top(E_{1;d}^\top + E_{m+2;d}) = I_d$. 
	\end{proof}
	We can now conclude the proof of our lemma. Let $L,\,R$ be as in Claim~\ref{claim:LDS_nilpotent}. We can readily verify that 
	\begin{align}
	\sigma_{\min}(L) = \sigma_{\min}(R) = 1, \label{eq:ssv_LR}
	\end{align}
	and additionally can write
	\begin{align*}
	\toep_{0,m+1,m+1}(G) &= \Diag(\underbrace{L,\dots,L}_{m+1 \text{ times }}) \,\cdot\,\powtoep_{m+1}(\nilp(G))\,\cdot\,\Diag(\underbrace{R,\dots,R}_{m+1 \text{ times }}),
	\end{align*}
	where we recall from Definition~\ref{defn:power_toep} that, for a square matrix $A$,
	\begin{align*}
	\powtoep_m(A) := \begin{bmatrix} I & A & A^2 & \dots & A^{m-1}\\
	0 & I & A & \dots & A^{m-2} \\
	\dots \\
	0 & 0 & 0 & \dots & I
	\end{bmatrix} 
	\end{align*}
	Therefore,
	\begin{align*}
	\sigma_{\min}(\toep_{0,m+1,m+1}(G)) &\ge \sigma_{\min}(L)\,\sigma_{\min}(\powtoep(\nilp_m(G)))\,\sigma_{\min}(R) \\
	&\overset{\text{by Eq.}\eqref{eq:ssv_LR}}{=} \sigma_{\min}(\powtoep(\nilp_m(G))).
	\end{align*} 
	We conclude the proof with the following upper bound on $\sigma_{\min}(\powtoep(\nilp_m(G)))^{-1}$:  applying Claim~\ref{claim:pow_toep_sigma_min}, and then Claim~\ref{claim:nilp_op} below,
	\begin{align*}
	\sigma_{\min}(\powtoep(\nilp_m(G)))^{-1} \le 1 + \opnorm{\nilp_m(G)} \le 1 +1 + \sum_{i=1}^{m} \opnorm{G^{[i]}}.
	\end{align*}
	\begin{claim}\label{claim:nilp_op} $\opnorm{\nilp_m(G)} \le 1 + \sum_{i = 1}^{m}\opnorm{G^{[i]}}$ 
	\end{claim}
	\begin{proof} We can write $\nilp_m(G)$ as the sum of two matrices: one containing the upper diagonal band of $1$'s, and the other the row of $G^{[m]},\dots,G^{[i]}$. The first matrix has operator norm one, and the second has operator norm at most $\sum_{i = 1}^{m}\opnorm{G^{[i]}}$. The claim now follows from the triangle inequality.
	\end{proof}
	The proof of the claim concludes our demonstration. \qed
